# Supplementary material for: OCSampler: Compressing Videos to One Clip with Single-step Sampling
Source: arXiv:2201.04388 source file (2022-01-12)
Supplement: Supplementary file 4 [file limitations.tex]

\section{Limitations}

The reward function in our framework is related to prediction results yielded from $f_{\textnormal{C}}$, thus the performance of classifier $f_{\textnormal{C}}$ will affect our sampling procedure.
